# Supplementary material for: Tracking Objects with 3D Representation from Videos
Source: arXiv:2306.05416 source file (2023-06-08)
Supplement: Supplementary file 2 [file kitti_impl.tex]

\begin{table}[]
\begin{center}
\resizebox{\linewidth}{!}{
\begin{tabular}{l|c}
\toprule
Configuration & Values\\
\midrule
optimizer & Adam\\
optimizer momentum &$\beta_1=0.9,\beta_2=0.999$ \\
weight decay & $1\times 10^{-5}$\\
learning rate &$8\times 10^{-5}$\\
learning rate scheduler &cosine decay \\
warmup iterations &500 \\
epochs &6+1+4 \\
augmentation &random flip, random resize [0.5,1.5] \\
aug. probability &0.5 \\
batch size &8 \\
gradient clip &5 \\
image size & 1920 $\times$1280 (zero padding)\\
\multirow{2}{*}{loss name} & heatmap loss, bbox loss, \\&depth loss, offset loss\\

loss weight & 1.0, 1.0, 0.2, 0.1  \\       
sync BN & True\\
\bottomrule
\end{tabular}}
\end{center}
\vspace{-10pt}
\caption{Implementation details of \methodname{} on KITTI dataset.}
\label{tab:kittiimpl}
\end{table}
