# Supplementary material for: Tracking Objects with 3D Representation from Videos
Source: arXiv:2306.05416 source file (2023-06-08)
Supplement: Supplementary file 3 [file oracle.tex]

\begin{table}[t]

   \begin{center}
    \resizebox{\linewidth}{!}{
        % \color{white}
        \begin{tabular}{l|ccccc}
            \toprule
                              & MOTA $\uparrow$    & IDF1 $\uparrow$    & FP $\downarrow$      & FN $\downarrow$      & ID Sw. $\downarrow$       \\
            \midrule
            \methodname{} (Ours) \\
            \textcolor{gray}{train w/ 3D GT}\\
            \textcolor{gray}{asso. w/ 3D GT}\\
            % SfM~\cite{schoenberger2016sfm} &55.5 &66.8 &55823 &249935 &11145 \\
            % MiDaS v3~\cite{Ranftl2022} &55.7 &63.4 &34514 &259471 &21058\\
            % MiDaS v3~\cite{Ranftl2022} + V.C.\\
            \bottomrule
        \end{tabular}
    }
    \end{center}
     \vspace{-10pt}
        \caption{Oracle experiments on KITTI \emph{training} set.}
    \label{tab:oracle}
\end{table}
