# Supplementary material for: Tracking Objects with 3D Representation from Videos
Source: arXiv:2306.05416 source file (2023-06-08)
Supplement: Supplementary file 4 [file wod_all.tex]

% \begin{table*}[]
% \resizebox{\linewidth}{!}{
% \begin{tabular}{lllllllllllllll}
% \toprule
%     & IDF1   & IDP    & IDR    & Rcll   & Prcn   & GT  & MT & PT & ML & FP   & FN   & IDs & FM  & MOTA \\
% \midrule
% cyclist & 45.3\% & 70.4\% & 33.4\% & 38.4\% & 81.0\% & 230 & 62 & 84 & 84 & 1060 & 7227 & 116 & 195 & 28.4\% \\
 
% \bottomrule
% \end{tabular}}
% \end{table*}

\begin{table*}[t]
   \begin{center}
    \resizebox{0.9\linewidth}{!}{
        % \color{white}
        \begin{tabular}{l|c|cc|ccccccccc}
            \toprule
            Method                 &Backbone                & Split & Category & MOTA $\uparrow$    & IDF1 $\uparrow$    & FN $\downarrow$      & FP $\downarrow$      & ID Sw. $\downarrow$ & MT $\uparrow$      & ML $\downarrow$            \\
            \midrule
            IoU baseline~\cite{lu2020retinatrack}    &ResNet-50    & val   & Vehicle  & 38.25              & -                  & -                    & -                    & -                   & -                  & -                              \\
            Tracktor++~\cite{bergmann2019tracking,lu2020retinatrack} &ResNet-50& val   & Vehicle  & 42.62              & -                  & -                    & -                    & -                   & -                  & -                                 \\
            RetinaTrack~\cite{lu2020retinatrack}    &ResNet-50     & val   & Vehicle  & 44.92              & -                  & -                    & -                    & -                   & -                  & -                                  \\
            QDTrack~\cite{fischer2022qdtrack}     &ResNet-50                              & val   & Vehicle  & 55.6               & 66.2               & 514548               & 214998               & 24309               & 17595              & 5559                            \\
            
            \methodname{} (Ours)&DLA-34 & val   & Vehicle &55.9 &65.6   &638390 &74802 &37478 &13643 &8583 \\
            \midrule
            QDTrack~\cite{fischer2022qdtrack}     &ResNet-50                              & val   & All      & 44.0               & 56.8               & 674064               & 264886               & 30712               & 21410              & 7510                               \\
            \methodname{} (Ours)\\
            \bottomrule
            % \toprule
            % Method                                 & Split & Category & MOTA/L1 $\uparrow$ & FP/L1 $\downarrow$ & MisM/L1 $\downarrow$ & Miss/L1 $\downarrow$ & MOTA/L2 $\uparrow$  & FP/L2 $\downarrow$ & MisM/L2 $\downarrow$ & Miss/L2 $\downarrow$ \\
            % \midrule
            % Tracktor~\cite{kim2018, waymo}         & test  & Vehicle  & 34.80              & 10.61              & 14.88                & 39.71                & 28.29               & 8.63               & 12.10                & 50.98                \\
            % CascadeRCNN-SORTv2*                    & test  & All      & 50.22              & 7.79               & 2.71                 & 39.28                & 44.15               & \textbf{6.94}      & 2.44                 & 46.46                \\
            % HorizonMOT*                            & test  & All      & 51.01              & 7.52               & 2.44                 & \textbf{39.03}       & \textbf{45.13}      & 7.13               & 2.25                 & \textbf{45.49}       \\
            % \midrule
            % QDTrack~\cite{fischer2022qdtrack} (ResNet-50)                       & test  & All      & 49.40              & \textbf{7.41}      & 1.46                 & 41.74                & 43.88               & 7.10               & \textbf{1.31}        & 48.21                \\
            % QDTrack~\cite{fischer2022qdtrack} (ResNet-101 + DCN)                & test  & All      & \textbf{51.18}     & 7.64               & \textbf{1.45}        & 39.73                & 45.09               & 7.20               & \textbf{1.31}        & 46.41                \\
            % \methodname{} (Ours)\\
            % \methodname{} (Ours)\\
            % \bottomrule
        \end{tabular}
    }
    \end{center}
    \vspace{-10pt}
        \caption{Results on WOD tracking \emph{val} set using py-motmetrics library.
    }
    \label{tab:waymo}
\end{table*}
